# Supplementary material for: Microscopic non-equilibrium energy transfer dynamics in a photoexcited metal/insulator heterostructure
Source: arXiv:1902.05264 ancillary file (2019-07-30)
Supplement: Supplementary file 1 [file rothenbach_supp.pdf]

# Supplementary information: Microscopic non-equilibrium energy transfer dynamics in a photoexcited metal/insulator heterostructure

N. Rothenbach,[1] M. E. Gruner,[1] K. Ollefs,[1] C. Schmitz-Antoniak,[2] S. Salamon,[1] P. Zhou,[1] R. Li,[3] M. Mo,[3] S. Park,[3] X. Shen,[3] S. Weathersby,[3] J. Yang,[3] X. J. Wang,[3] R. Pentcheva,[1] H. Wende,[1] U. Bovensiepen,[1,*] K. Sokolowski-Tinten,[1] and A. Eschenlohr[1,†]

[1]*Faculty of Physics and Center for Nanointegration (CENIDE), University of Duisburg-Essen, Lotharstr. 1, 47057 Duisburg, Germany*
[2]*Forschungszentrum Jülich, Wilhelm-Johnen-Str., 52428 Jülich, Germany*
[3]*SLAC National Accelerator Laboratory, 2575 Sand Hill Rd., Menlo Park, California 94025, USA*
(Dated: July 30, 2019)

## I. SAMPLE PREPARATION

The investigated $[Fe/MgO]_n$ heterostructures were grown by molecular beam epitaxy. The substrate consists of a 200 nm thick $Si_3N_4$ membrane, with a 100 nm thick Cu heat sink, which was grown beforehand by molecular beam epitaxy on its backside. Before the growth of either the heat sink or the heterostructure, the substrate was heated up to 600 K for 30 min to eliminate $H_2O$ and other possible contaminations on the substrates. During material growth the substrate was held at 400 K in a background pressure of $10^{-10}$ mbar to avoid oxidation and maintain the purity of the individual deposited layers. The $Si_3N_4$ substrate leads to growth of polycrystalline Fe and MgO layer stacks. The thicknesses of the individual polycrystalline layers were monitored during growth by a quartz-crystal microbalance and subsequently determined by small angle x-ray diffraction.

Fig. S1 shows an exemplary small angle x-ray diffractogram of a $[Fe/MgO]_n$ heterostructure with $n = 8$ layer stacks with a nominal thickness of 2 nm of the single layers. In its inset a schematic representation of the composition of the multilayer is depicted. The measured diffractograms were fitted using layer thicknesses of $2.30 \pm 0.01$ nm, $2.30 \pm 0.01$ nm and 200.00 nm for Fe, MgO and $Si_3N_4$, respectively, confirming our thicknesses.

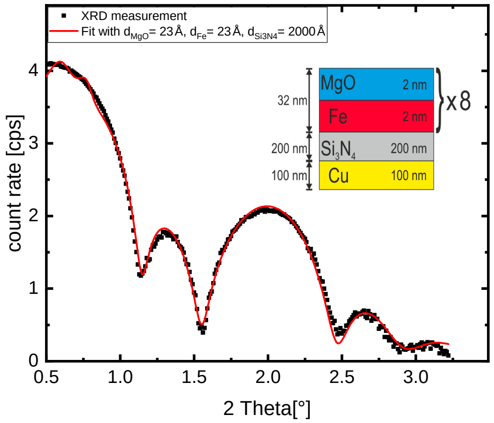


FIG. S1. Small angle x-ray diffraction measurement of a $[Fe/MgO]_8$ heterostructure. The inset shows a schematic representation of the composition of the multilayer sample.

## II. INTERFACE QUALITY

In order to determine the quality of the Fe-MgO interfaces, two test samples were fabricated. In both of these, one of the Fe layers of 2 nm nominal thickness was replaced by a layer composed of 1.4 nm natural Fe and 0.6 nm of pure $^{57}Fe$, referred to as tracer layer. One sample (single stack) consisted of only one Fe-MgO layer pair, with the tracer layer located at the interface between the two, while the second sample (fourfold stack) had the tracer layer located at the topmost interface in a fourfold stack of Fe-MgO layer pairs. This was done in order to check for any effects such as increased roughness of the interface after a multitude of layers, compared to only one layer pair.

Conversion electron Mössbauer spectroscopy (CEMS) measurements were carried out on both samples at room temperature, with the results being shown in Fig. S2. It is reasonable to assume that the predominant signal observed in these spectra is being produced by the tracer layer, due to the comparatively low occurrence of $^{57}Fe$ in natural Fe (ca. 2 % [1]). To evaluate the obtained spectra, and to determine the amount of signal being generated by $^{57}Fe$ atoms that potentially diffused into the MgO layer, the following procedure was used: The dominant sextet contribution (blue), stemming from $^{57}Fe$ atoms that are exclusively surrounded by other Fe atoms, was fitted with a distribution of equidistant sextet subspectra, using typical parameters for bcc-Fe. Applying upper and lower limits corresponding to the main peak of the hyperfine field distribution ensured that only the spectral contribution of the dominant bcc-Fe sextet was taken into account by this data fit.

The entire rest of the spectrum can be assumed to originate from $^{57}Fe$ atoms that have different nearest neigh-

* uwe.bovensiepen@uni-due.de
† andrea.eschenlohr@uni-due.de

bors, resulting from interdiffusion into the MgO layer, leading to different magnetic hyperfine fields. To consider this, free distributions of hyperfine fields (green) were utilized to account for the entirety of the spectral area not covered by the bcc-Fe sextet (blue). Furthermore, a very small percentage of $^{57}$Fe atoms shows paramagnetic behavior, leading to a miniscule singlet (cyan) at the center of the spectrum. We can assume this contribution to stem from a small number atoms that have diffused so far into the MgO layer that they lack a relevant number of Fe nearest neighbors, thus not showing any magnetic ordering. Utilizing the sum of these contributions as a worst-case approximation, we can use the total relative spectral area stemming from the interdiffused atoms to determine an effective thickness of this interdiffusion zone relative to the nominal thickness of the 0.6 nm tracer layer. This provides us with an estimate of the effective thickness of the interdiffusion zone of $0.19 \pm 0.01$ nm for the single Fe-MgO layer pair and $0.17 \pm 0.01$ nm for the fourfold layer pairs, clearly showing that the higher number of stacked layers does not have any kind of detrimental effect on the quality of the interface.

It has to be stressed that this is an absolute worst-case assumption. In case of a theoretically perfect interface, the $^{57}$Fe atoms that are at the edge of the Fe layer would still produce deviating hyperfine magnetic fields due to the MgO nearest neighbors to one side. Our approximation thus also includes these atoms into the spectral area of the interface, even if no interdiffusion has taken place. The quality of the interface can therefore only be higher than what our estimate provides here. From the obtained results, we can thus conclude that even in the worst case, potential intermixing of the constituents does not significantly exceed an effective thickness of one monolayer at the Fe-MgO interfaces, which are therefore considered to be atomically sharp.

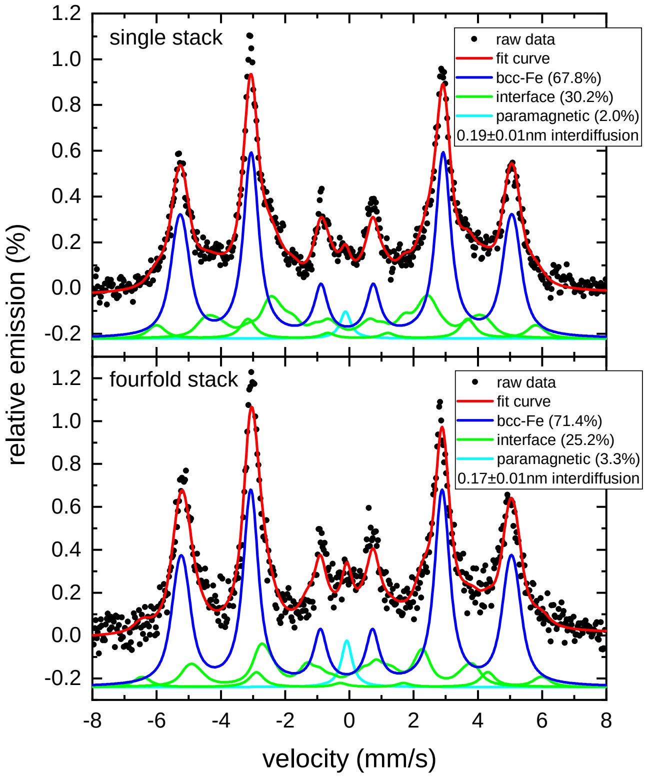


FIG. S2. Conversion electron Mössbauer spectroscopy (CEMS) measurements on two test samples at room temperature. For more details see text.

## III. REFERENCE MEASUREMENTS: MGO

To ensure that the dynamics observed by time-resolved x-ray absorption spectroscopy (XAS) at the O K edge are mediated by the Fe constituent in the heterostructure and not by a different effect resulting directly from the MgO itself (e.g. caused by multi-photon absorption of the pump pulse), we carried out femtosecond (fs) XAS on a 16 nm thick polycrystalline MgO reference film. The reference sample was grown by molecular beam epitaxy on the same substrate and under the same preparation conditions as the corresponding heterostructure (see above). Therefore, we can exclude any influence of the sample quality on the measurements.
In order to compare the time-dependent O K edge absorption signals for the heterostructure and the reference sample we optically excited both samples with the same UV pumping as described in the manuscript ($h\nu = 4.7$ eV, incident fluence $\approx 20$ mJ/cm$^2$). Fig. S3 shows that the MgO reference sample exhibits no pump-induced changes after laser excitation. Thus, the absence of a transient XAS signal at the pure MgO sample demonstrates that the observed changes at the O K edge in our $[\mathrm{Fe/MgO}]_n$ heterostructure are interface-mediated dynamics, driven by excitation of the Fe constituent.

## IV. REFERENCE MEASUREMENTS: FE

We measured fs time-resolved XAS at the Fe $L_3$ edge of a 20 nm Fe reference sample and compared it to the pump-induced response of the $[\mathrm{Fe/MgO}]_n$ heterostructure ($n = 8$), see Fig. S4. We find qualitative differences in the pump-induced changes observed in these samples, which we ascribe to the role of energy transfer across the Fe/MgO interface, as discussed in the main manuscript. In the heterostructure, an ultrafast increase followed by a decay and subsequent, slower increase in the time-dependent XAS signal is observed. Together, this results in a local minimum of the pump-induced change at about 1.2 ps, which is absent in the bulk-like Fe reference sample. The reference sample exhibits simpler dynamics with an increase and decay.

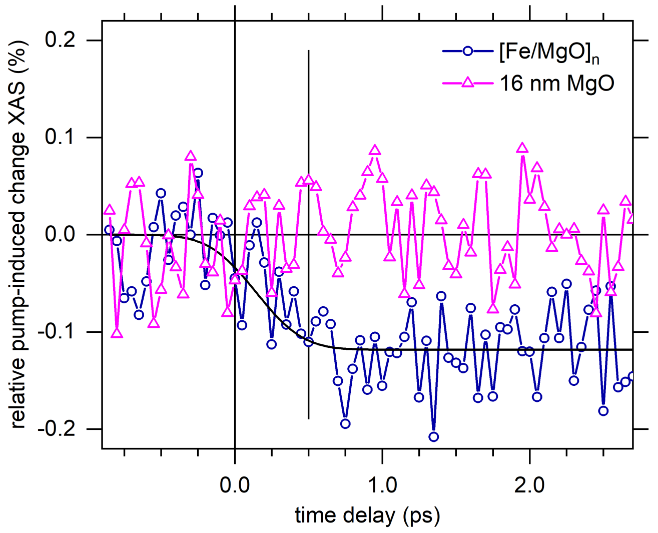


FIG. S3. Pump-induced changes observed at the O K edge of the [2 nm Fe/2 nm MgO]$_n$ heterostructure ($n$ = 8) and a 16 nm MgO reference sample as a function of the pump-probe delay.

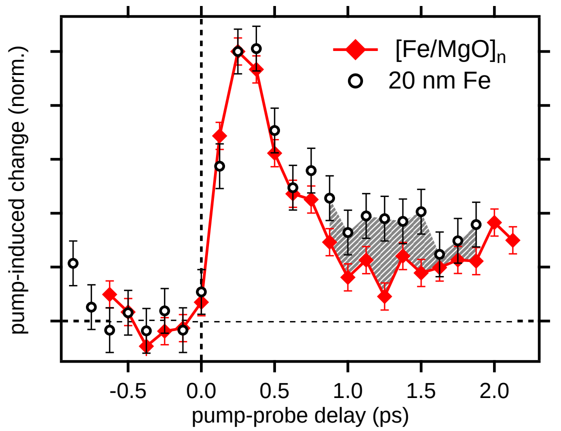


FIG. S4. Pump-induced changes observed at the Fe $L_3$ edge of the [2 nm Fe/2 nm MgO]$_n$ heterostructure ($n$ = 8) and a 20 nm Fe reference sample as a function of the pump-probe delay. The [Fe/MgO]$_n$ data were interpolated to obtain the same number of data points as for 20 nm Fe for a better comparison. The data are normalized to the pump-induced change at 0.2 ps due to the difference in the initial rise of the signal.

## V. REFERENCE MEASUREMENTS: PICOSECOND TIME-RESOLVED XAS

In Fig. S5 below, we compare the spectral changes at the O K edge of the [Fe/MgO]$_n$ heterostructure in the sub-ps range to those at 90 ps pump-probe delay, when the phonon system has equilibrated and the heterostructure as a whole has thermalized. Fig. S6 further shows the pump fluence dependence of the spectral changes at the O K and Fe $L_3$ edges at 90 ps pump-probe delay after excitation with UV pulses ($h\nu = 4.7$ eV).

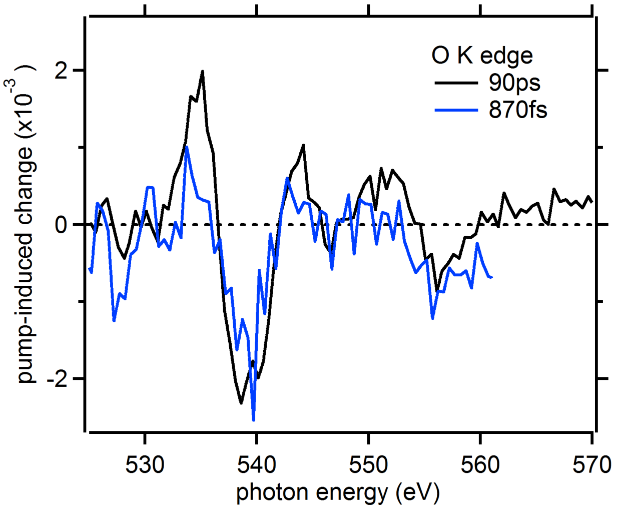


FIG. S5. Pump-induced changes at the O K edge of a [Fe/MgO]$_n$ heterostructure at the indicated pump-probe delays after 4.7 eV laser excitation. The fs data were acquired with about 150 fs time resolution in Femtoslicing mode, while the 90 ps data were acquired with about 70 ps time resolution.

## VI. DETAILS OF THE CALCULATIONS

The calculations of a $Fe_8/(MgO)_8(001)$ heterostructure were carried out in the framework of density functional theory (DFT) using the generalized gradient approximation (GGA) in the formulation of Perdew, Burke and Ernzerhof (PBE) [2]. First, structural optimization of the 24 atom primitive cell with respect to atomic positions and lattice parameters was carried out with the VASP code [3, 4] using PAW potentials with the electron configurations $3p^6 3d^7 4s^1$ for Fe, $2p^6 3s^2$ for Mg and $2s^2 2p^4$ for O and an energy-cutoff of 580 eV. Results were considered converged, when the energy fell below $10^{-8}$ eV between two consecutive electronic and $10^{-6}$ eV between two geometric optimization steps. Brillouin zone integration was carried out on 90 $k$-points in the irreducible zone (IBZ) in combination with a Gaussian-type Fermi-surface smearing with a width of $\sigma = 0.1$ eV. For the electronic DOS we applied the tetrahedron method with Blöchl-corrections [5] and 408 $k$-points for the Brillouin-zone integration.

The phonon dispersion and vibrational density of states was determined with the so-called direct approach based on the restoring forces obtained from central differences between $2 \times 24$ displacements of inequivalent atoms in a 768 atom supercell, constructed as a $4 \times 4 \times 2$ replication of the 24 atom primitive cell. Here, a k-mesh of $5 \times 5 \times 1$ points in the full Brillouin zone (FBZ) in combination with Gaussian smearing of width $\sigma = 0.05$ eV was employed which guarantees the required accuracy. Finally the dynamical matrix and the vibrational density of states was obtained after employing the PHON code by Dario Alfè [6].

Full layer-resolved calculations of the electronic and

vibrational density of states can be found in Figs. S7 and S8, respectively. The response of the electronic density of states to uniaxial lattice compression and expansion is displayed for all layers of the heterostructure in Fig. S9.

X-ray absorption spectra were calculated with the fully-relativistic SPRKKR Korringa-Kohn-Rostoker multiple scattering approach [7, 8] using the optimized structure obtained in the previous step. Contour integration was carried on an arc with 48 energy points, 1134 $k$-points in the IBZ and an angular momentum expansion included $d$-states until the convergence criterion of $10^{-6}$ Ry was achieved. The spectra were obtained within the independent particle approximation. They were broadened with a Lorentzian with a width of 0.2 eV and shifted on the energy scale by a constant offset to match the experimental peak at 540 eV.

[1] P. Gütlich, E. Bill, and A. Trautwein, *Mössbauer Spectroscopy and Transition Metal Chemistry* (Springer-Verlag GmbH, Heidelberg, 2011).
[2] J. P. Perdew, K. Burke, and M. Ernzerhof, Phys. Rev. Lett. **77**, 3865 (1996).
[3] G. Kresse and J. Furthmüller, Phys. Rev. B **54**, 11169 (1996).
[4] G. Kresse and D. Joubert, Phys. Rev. B **59**, 1758 (1999).
[5] P. E. Blöchl, O. Jepsen, and O. K. Andersen, Phys. Rev. B **49**, 16223 (1994).
[6] D. Alfè, Comp. Phys. Commun. **180**, 2622 (2009).
[7] SPR-KKR, version 7.7, H. Ebert et al, http://olymp.cup.uni-muenchen.de/ak/ebert/SPRKKR.
[8] H. Ebert, D. Ködderitzsch, and J. Minár, Rep. Prog. Phys. **74**, 096501 (2011).

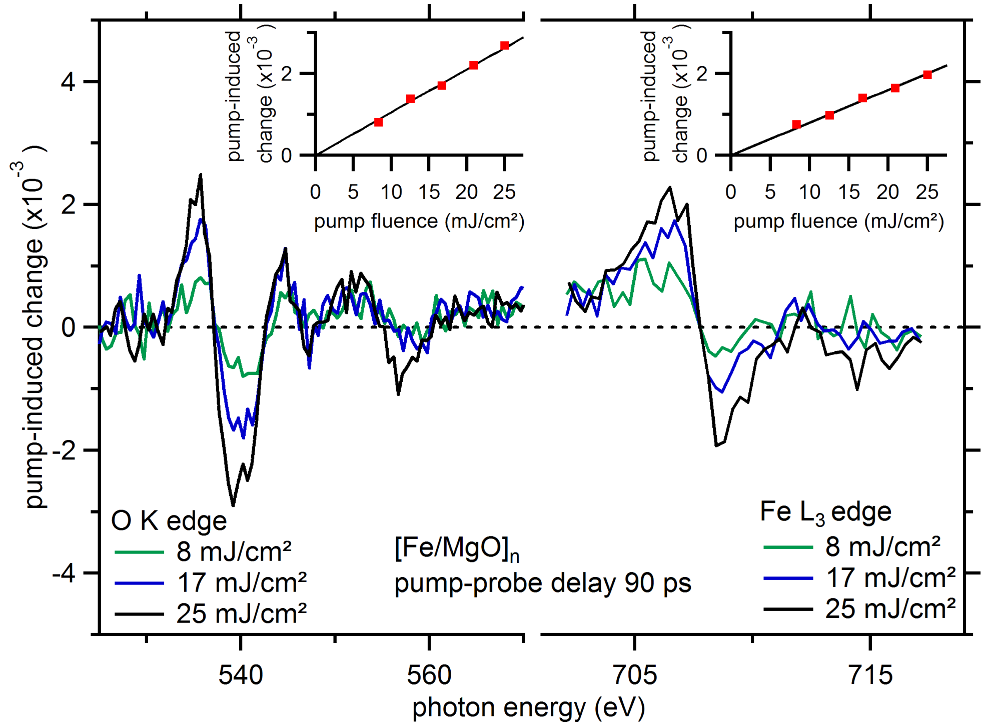


FIG. S6. Pump-induced changes at the O K edge (left) and Fe $L_3$ edge (right) of a $[Fe/MgO]_n$ heterostructure at a pump-probe delay of 90 ps after 4.7 eV laser excitation with the indicated pump fluences. The data were acquired with a time resolution of about 70 ps. The insets show a linear relation between the amount of pump-induced change, defined as half of the peak-to-peak value, and the pump fluence.

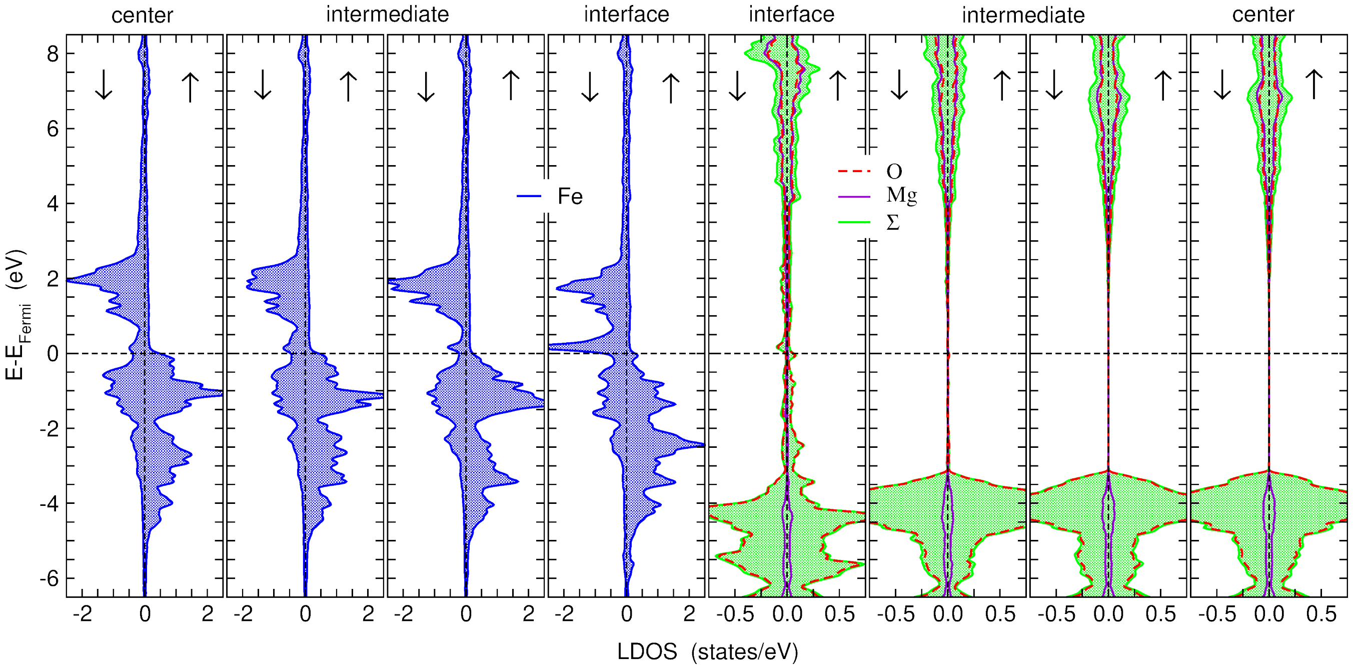


FIG. S7. Spin-polarized element- and layer-resolved electronic density of states of $Fe_8/(MgO)_8(001)$ obtained from DFT calculations. The contribution of Fe is represented by the blue lines, Mg by purple lines and O by the dashed red lines. The sum of Mg and O contributions is indicated by the green area. Upward and downward arrows denote the respective spin channels.

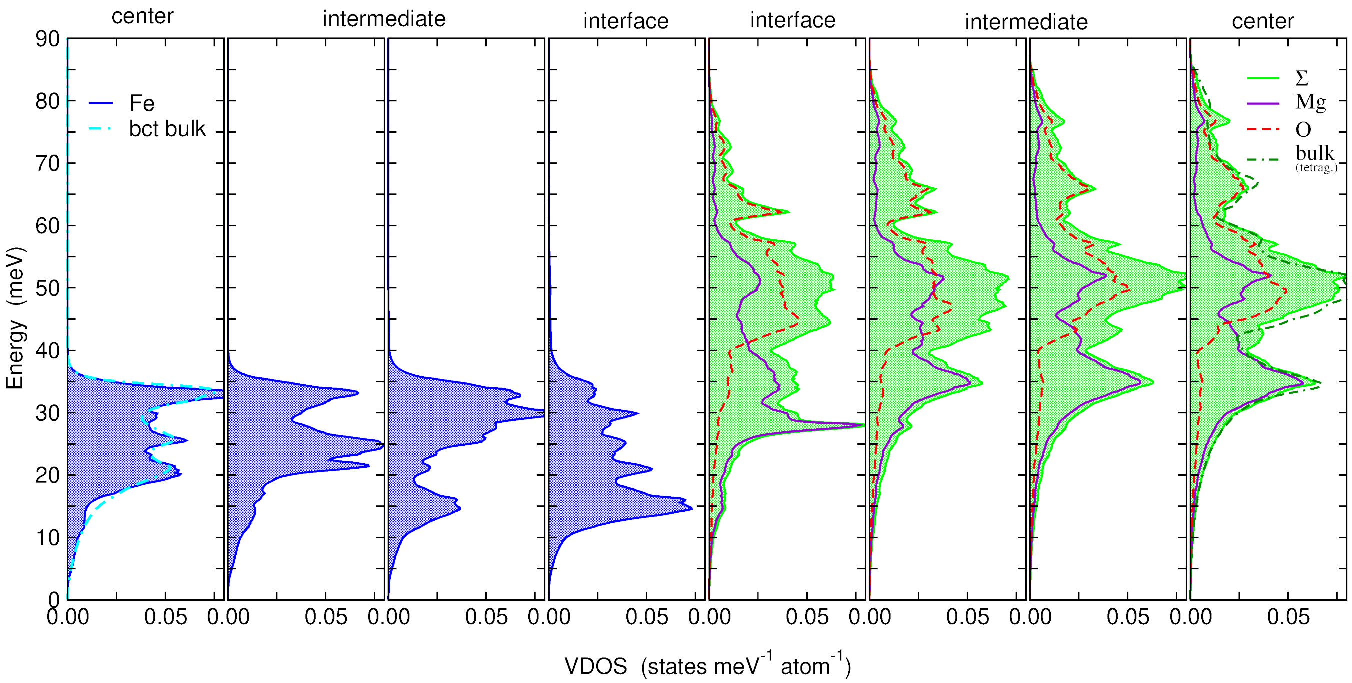


FIG. S8. Layer-resolved vibrational density of states of $Fe_8/(MgO)_8(001)$obtained from DFT calculations. Colors and symbols as in Fig. S7. In all layers O predominantly contributes at energies above 40 meV, where Fe-modes are not encountered anymore. The interface layers are characterized by the hybridization between Fe and Mg in the optical modes.

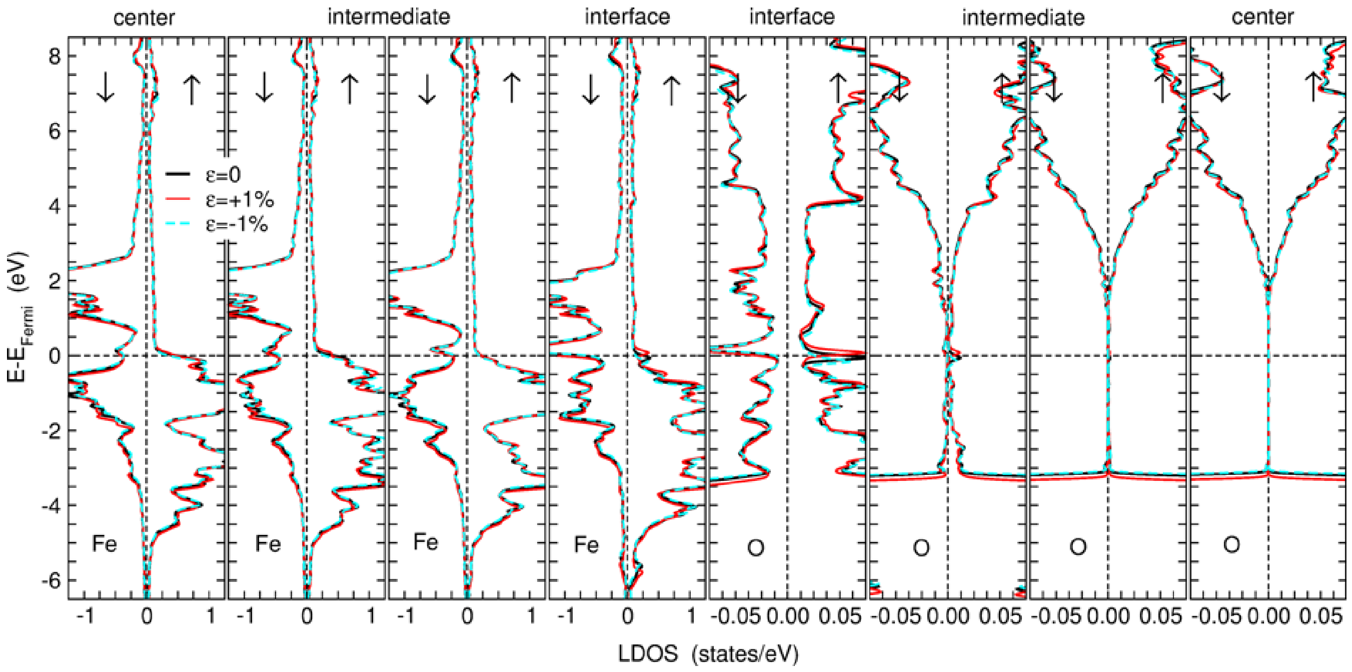


FIG. S9. Layer-resolved electronic density of states under 1% compression (red line) and expansion (blue, dashed line) of $Fe_8/(MgO)_8(001)$ at the Fe-MgO interface obtained from DFT calculations.
